# Supplementary material for: Mechanism of feature learning in convolutional neural networks
Source: arXiv:2309.00570 source file (2023-09-01)
Supplement: Supplementary file 1 [file laplace_cntk.tex]

\section{Laplace CNTK}
\label{app:laplace_cntk}

We introduce an alternative convolutional kernel derived from the traditional Laplacian kernel. This kernel has the following form:
\begin{definition}[Convolutional Laplace kernel]
For $x, x' \in \mathbb{R}^d$, composed of patches of size $q$ and indexed $p \in P$, we define the (Mahalanobis) Convolutional Laplace kernel $k: \Real^d \times \Real^d \rightarrow \Real$ with bandwidth $L$ and Mahalanobis matrix $M \in \Real^{q \times q}$ by:
\begin{align*}
    k(x,x') = \sum_{p \in P} \exp\round{-L\|x_{[p]} - x_{[p']}\|_M}
\end{align*}
\end{definition}
Notably, we can obtain a significant performance improvement on CIFAR-10/100 using the AGOP from ReLU-CNTK with Laplace kernel ConvRFM. We refer to this combined method as Laplace::ConvRFM (Figure~\ref{fig: LaplaceCNTK Cifar}).
\begin{figure}[h]
    \centering
    \includegraphics[width=0.75\textwidth]{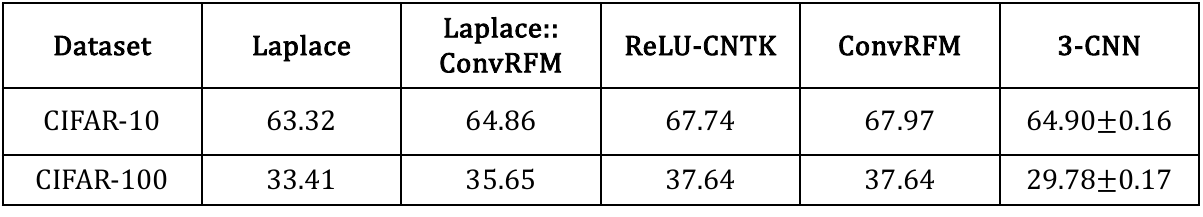}
    \caption{Performance improvement with Laplace::ConvRFM on CIFAR datasets.}
    \label{fig: LaplaceCNTK Cifar}
\end{figure}
For these experiments, we took the $M$ matrix from the second iteration of (shallow) CRFM with ReLU-CNTK. We used a fixed bandwidth of $L=10$ and tuned regularization among $10^{-3}$, $10^{-9}$ for the convolutional Laplace kernel.
